# Supplementary material for: PEM: Representing Binary Program Semantics for Similarity Analysis via a Probabilistic Execution Model
Source: arXiv:2308.15449 source file (2023-08-30)
Supplement: Supplementary file 1 [file suppl-old.tex]

\section{Ablation Study}
\xx{I put a draft version on the website: https://paper-authors.github.io}
We conduct three ablation studies to analyse how each part of our system contributes to the results. They are focused on the path sampling algorithm, the selection of input seed values, and the distribution of generated observable values, respectively. All the studies are conducted on the main functions of Coreutils, compiled with {\tt O0} and {\tt O3}, respectively. We run \toolname with different configurations and compare each main function in {\tt O3} against every main function in {\tt O0}. We use PR@1 and code coverage as metrics in the ablation study.

\subsection{Path Sampling}

The space of program paths is enormous. Thus it is important to extract enough semantic behaviors from a limited number of paths. In this study, we change the number of paths we want to explore for a function and the largest $k$ in $k$-edge-off paths. The results are shown in Table~\ref{tab:abl:mutate}. The first column lists the number of paths we want to explore, the second one is the largest $k$, the third to fifth columns are the PR@1, the coverage for {\tt O0} functions and the coverage for {\tt O3} functions, respectively.
We run the experiments with the five sets of configurations where the third one (marked in bold) \xz{do you mean the third?\xx{Fixed}} is the configuration we use for evaluating other RQ's\xx{I attempted to say we use the third config to conduct the other parts of the evaluation. Thus maybe here should be RQs meaning research questions? }.



\begin{table}[h]
    \centering
    \caption{Ablation Study on Path Sampling}
    \label{tab:abl:mutate}
    \begin{tabular}{c|c|c|c|c}
        \#Path & $k$ & PR@1 & Cov-O0 & Cov-O3 \\
        \hline
        1 & 0 & 92.2     &  0.55    & 0.30 \\
        40 & 1 & 94.2   &  0.64    & 0.45 \\
        \textbf{400} & \textbf{2} & \textbf{95.1}   &  \textbf{0.74}    & \textbf{0.58}  \\
        4000 & 3 & 95.1  &  0.82    & 0.65 \\
        4000 & INF & 95.1  &  0.82    & 0.66  \\
    
    \end{tabular}
\end{table}



The first configuration sets the path number to 1 and $k$ to 0. With this configuration, \toolname faithfully interprets one path without flipping any predicate. 
While it achieves a PR@1 of 92.2, it covers only 55\% code in O0 functions and only 30\% in O3 functions. Note that the main functions in Coreutils typically have a larger number of checks for input formats. Thus a significant amount of the covered code is for error processing. 

When we slightly increase the number of paths (to 40) and set $k$ to 1, the coverage for {\tt O0} and {\tt O3} functions increases by 10\% and 15\%, respectively. Also, the PR@1 increases by 2\%. That indicates our path sampling strategy cannot only  effectively cover more code, but also consistently select corresponding paths that generate similar values among similar functions. 
We further increase the max number of paths to 400 and set $k$ to 2. \toolname achieves better performance in both PR@1 and coverage. When $k$ is larger than 2, 
while the code coverage increases, the change on PR@1 is marginal.
The PR@1 is not 100\% because during some optimizations, the compiler selects instructions that have not been modeled in our system.

\smallskip\noindent{\bf Conclusion}: Our path sampling strategy significantly improves code coverage in both {\tt O0} and {\tt O3} programs. It samples consistent sets of paths among optimized and unoptimized programs. However, $k>2$ can only achieve marginal improvement on the final results.


\subsection{Selection of Seed Inputs}
\label{sec:abl:value-dist}

To see how \toolname performs with different seed inputs, we run our system with 10 different sets of seed values. The performance is depicted in Fig.~\ref{fig:seed-value}. The horizontal axis marks the metrics, i.e., PR@1, code coverage for O0, and code coverage for O3. The vertical axis shows the percentage value. We can see that all the three metrics fluctuate less than 10\% across different seed values.
Even if we consider the worst case for each metric, \toolname still achieves good performance with PR@1 of 92\%, and code coverage of 74\% and 58\% for {\tt O0} and {\tt O3} binary programs, respectively.
There are two major causes of the variation: different seed values may trigger different seed paths; different seed values have different properties under some operations. For example, consider the expression {\tt x\&1} and {\tt x\&5}, where {\tt\&} denotes the bitwise-and operation. They yield the same results when {\tt x=9}, while they yield different results if {\tt x=7}. 
\begin{figure}
    \centering
    \includegraphics[width=.3\textwidth]{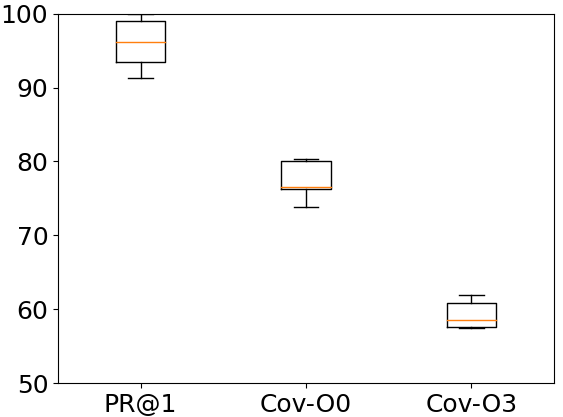}
    \caption{Variances w.r.t. Seed Inputs}
    \label{fig:seed-value}
\end{figure}

\smallskip\noindent{\bf Conclusion}: The performance of \toolname has only small variance under different seed inputs. It consistently achieves good performance regardless of values of seed inputs.


\subsection{Distribution of Observable Values}

In this ablation study, we investigate whether matched values (i.e., values appearing in both optimized and unoptimized programs) have similar frequencies in both the {\tt O0} programs and the {\tt O3} programs.
We use the function pair {\it dd} and {\it mv} as an example. The results are visualized in Fig.~\ref{fig:value_freq}. There are four plots in Fig.~\ref{fig:value_freq}. They are the match results between {\it dd-O0} and {\it dd-O3}, {\it mv-O0} and {\it dd-O3}, {\it dd-O0} and {\it mv-O3}, and {\it mv-O0} and {\it mv-O3}, respectively.  For each plot, the horizontal axis and the vertical axis mark the frequency of values in the {\tt O0} and {\tt O3} programs, respectively. As marked within the orange boxes, under our sampling method, most matched values between two similar functions have a matching frequency before and after optimization. In contrast, for the dissimilar function pairs, even though some of their matched values also have a matching frequency, a significant part of them have very different distributions before and after optimization.

\smallskip\noindent{\bf Conclusion}: The frequency of output values are significant to reveal the semantics of programs. The sampling algorithm of \toolname can consistently sample values from similar functions with similar frequency and can effectively distinguish values from dissimilar functions.

\begin{figure}
    \centering
    \includegraphics[width=.40\textwidth]{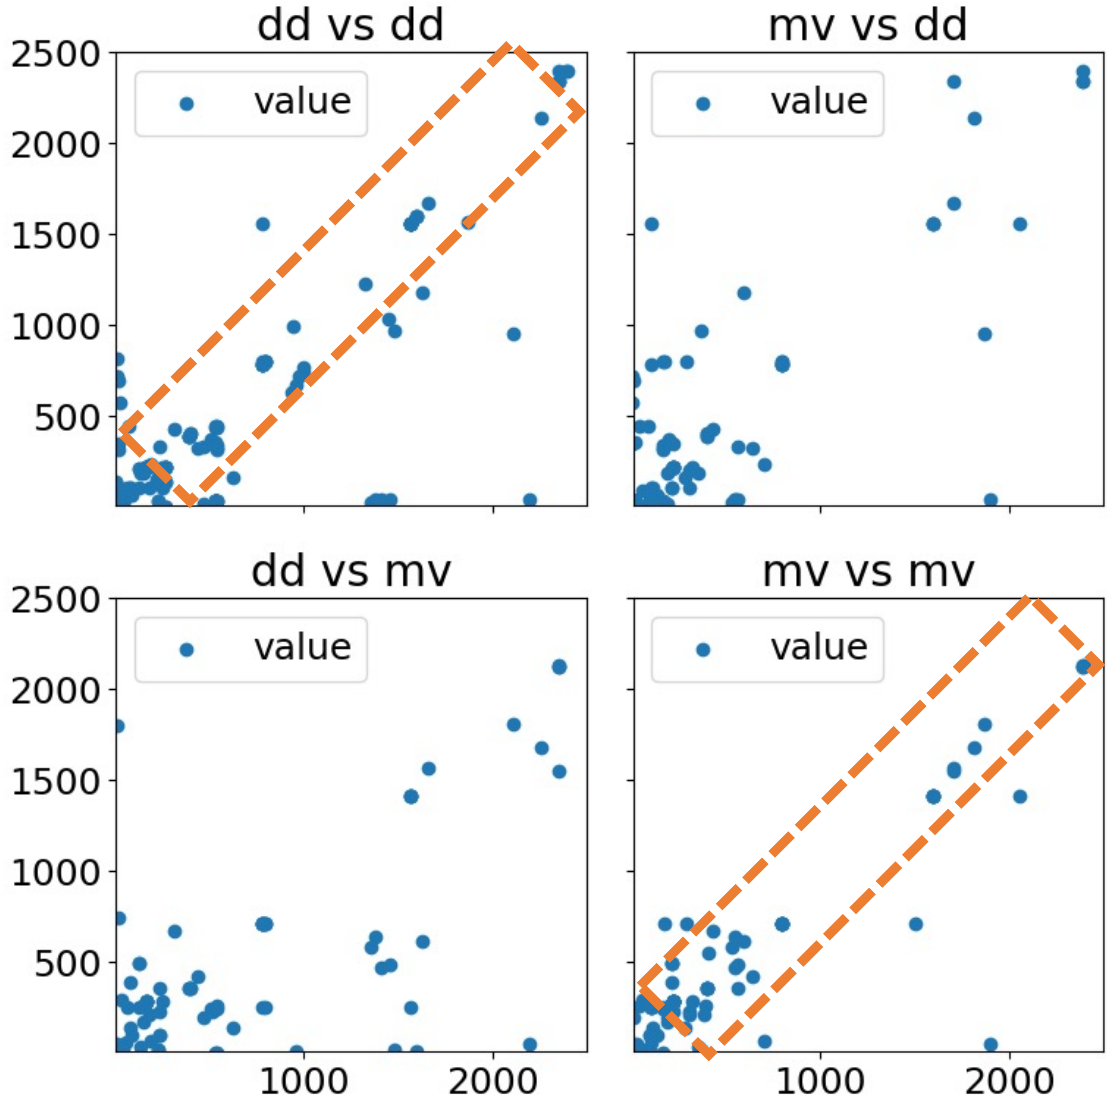}
    \caption{Distribution of Matched Values}
    \label{fig:value_freq}
\end{figure}





\section{Case Study}
We conduct a case study to use different binary similarity detection tools to find 1-day vulnerabilities.
The study is conducted with 10 CVEs. For each CVE related function, we query with the function compiled by {\tt O3} in the whole {\tt O0} binary program consisting of all functions in the related project. Then we record the ranking of the ground truth function.

The results are listed in Table~\ref{tab:case-study}. The first three columns are the CVE ID, the related projects, and the number of functions in the project, respectively. The fourth column lists the name of the function related to the CVE. The last three columns show the ranking of the ground truth function predicted by the tools. Note that an X in the last three columns means the related tool cannot find the problematic function within the top 200 matched functions.  \toolname finds most CVEs with the highest rank. It only misses {\tt CVE-2016-9842} in Zlib. We investigate the related function and find it is a very small function with only 30 instructions. There are very few observable values. Thus our system does not capture enough semantics for this function.
The two ML-based methods list the problematic function with the highest rank in only 1 case. If we consider functions ranking in the top 30, both of them can successfully find 2 more problematic functions.

\smallskip\noindent{\bf Conclusion}: \toolname can effectively find problematic functions in real-world scenarios with significantly fewer false positives than the ML-based methods. Especially, \toolname performs better when the problematic function has relatively complex semantics. On the other hand, when a function is too simple for \toolname to capture enough semantic features, ML-methods can help detect it.


\begin{table*}
\caption{Searching for
One-Day Vulnerabilities\xx{Vertical lines are broken. We'll fix it when make the website.} }
\label{tab:case-study}
\centering
\small
\begin{tabular}{r|l|l|l|ccc}
\toprule
\multirow{2.5}{*}{\textbf{CVE}} & \multirow{2.5}{*}{\textbf{\begin{tabular}[c]{@{}c@{}}Project \\ Name\end{tabular}}} & \multirow{2.5}{*}{\textbf{\# Functions}} & \multirow{2.5}{*}{\textbf{\begin{tabular}[c]{@{}c@{}}Function \\ Name\end{tabular}}} & \multicolumn{3}{c}{\textit{\textbf{Result}}} \\ \cmidrule(lr){5-7} 
 &  &  &  & \multicolumn{1}{c}{\textbf{SAFE}} & \multicolumn{1}{c}{\textbf{Trex}} & \textbf{\toolname{}} \\ \midrule
CVE-2017-18018 & Coreutils & 931 & chown & \multicolumn{1}{c}{10} & \multicolumn{1}{c}{72} &  1 \\ \hline
CVE-2007-2452 & Findutils(locate) & 97 & visit\_old\_format & \multicolumn{1}{c}{X} & \multicolumn{1}{c}{28} &  1\\ \hline
CVE-2021-20311 & ImageMagick & 1702 & sRGBTransformImage & \multicolumn{1}{c}{152} & \multicolumn{1}{c}{X} & {\color{red}43}\xx{TBD} \\ \hline
CVE-2021-20309 & ImageMagick & 1702 & WaveImage & \multicolumn{1}{c}{34} & \multicolumn{1}{c}{X} &  1\\ \hline
CVE-2019-13308 & ImageMagick & 1702 & ComplexImages & \multicolumn{1}{c}{79} & \multicolumn{1}{c}{X} &  1 \\ \hline
CVE-2016-9842 & Zlib & 91 & inflateMark & \multicolumn{1}{c}{30} & \multicolumn{1}{c}{1} & 1 \\ \hline
CVE-2021-4044 & Openssl & 2653 & X509\_verify\_cert & \multicolumn{1}{c}{X} & \multicolumn{1}{c}{5} & 1 \\ \hline
CVE-2021-3711 & Openssl & 2653 & EVP\_PKEY\_decrypt & \multicolumn{1}{c}{114} & \multicolumn{1}{c}{43} & 1 \\ \bottomrule
\end{tabular}
\end{table*}
